# Supplementary material for: Incremental Few-Shot Instance Segmentation
Source: arXiv:2105.05312 source file (2021-05-11)
Supplement: Supplementary file 1 [file Supplemental.pdf]

# Incremental Few-Shot Instance Segmentation – Supplementary Material


Dan Andrei Ganea
Utrecht University
dan.andrei.ganea@gmail.com

Bas Boom
Cyclomedia Technology
bboom@cyclomedia.com

Ronald Poppe
Utrecht University
r.w.poppe@uu.nl


## 1. Confidence intervals for reported results

We report the 95% confidence intervals for the main results in the paper. Specifically, Tables 1 and 2 report on the COCO-All evaluation scenario for few-shot object detection and few-shot instance segmentation, respectively. These results supplement those in Table 1 in the main paper.

For the COCO-Novel evaluation scenario (Table 2 in the paper), we provide 95% confidence intervals in Table 3. The performance relative to other methods, and consequently our conclusions, are not affected by this mistake. We additionally report AP75 performance.

The comparison between MTFA/iMTFA and Siamese Mask R-CNN on COCO-Split-2 appears in Table 4. Finally, the results including confidence intervals for the COCO2VOC evaluation setting appear in Table 5 (Table 4 in the paper). In both tables, we also report AP75 performance for detection and segmentation.

## 2. Per-class detection and segmentation results

Table 6 summarizes the detection and segmentation performance, including 95% confidence intervals, on the COCO novel classes. The results are sorted in decreasing order on the segmentation AP. Clearly, classes with less variation in object appearance (e.g., `TV`, `bus`, `car`) are better detected and segmented than classes with more variation (e.g., `person` and `dining table`). For the `person` class, the articulation of the body introduces significant challenges. In addition, COCO contains many images with small instances of people, typically in the background. For the `dining table` class, many false positives occur as items that are associated with food are incorrectly classified as a dining table. Paradoxically, `dining table` masks are annotated to be the areas of the table excluding those of the objects on the table such as plates, cutlery, hands and food. Since our mask prediction head is trained in a class-agnostic manner, such subtleties are overlooked. Example results for the `dining table` class also appear in Figure 4 (bottom row, images 4–5) of the paper.

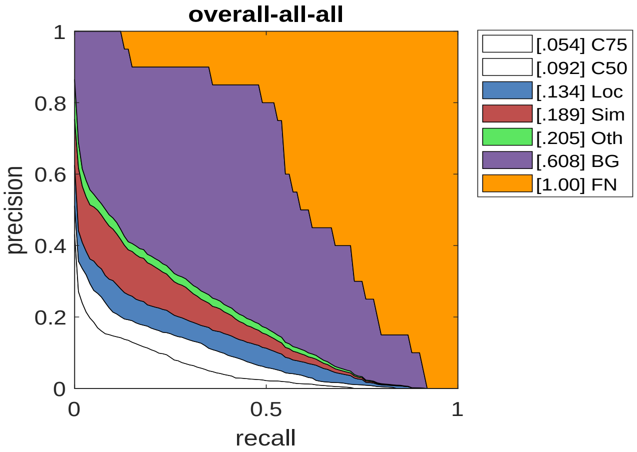


Figure 1. **Precision-recall curve for instance segmentation on the COCO novel classes.** See Section 3 for an explanation of the labels.

## 3. Per-class precision-recall curves

In Figure 1, we show the precision-recall (PR) curve for all COCO novel classes. The curves are inspired by Hoiem *et al.* [1] and generated using COCOAPI.

The resulting PR curves represent a series of 7 evaluation settings, each obtaining a higher or equal AP to the previous one. 'C75'and 'C50' stand for AP75 and AP50, while 'Loc' represents AP10. The 'Loc' setting ignores localization errors. The 'Sim' and 'Oth' curves represent precision ignoring class confusions from the same super-category and from all categories, respectively. Finally, the 'BG' curve ignores all background confusions, while the 'FN' curve represents all false negatives.

The high overall precision obtained for 'BG' shows that our model overly detects classes as background. Since the class representative for the background is taken directly from the training on the base classes, it can be close to the novel class representatives in our learned metric space.

The 20 COCO novel classes are split into 7 of the 11 predefined COCO super-categories. Results on these appear in Figure 2. We use the seed out of 10 random seeds that achieved an AP closest to the mean of these seeds.

| Shots | Inc. | Method | Detection | | | | | |
|---|---|---|---|---|---|---|---|---|
| | | | Overall | | Base | | Novel | |
| | | | **AP** | **AP50** | **AP** | **AP50** | **AP** | **AP50** |
| 1 | | Base-Only | **28.67** | **43.53** | **38.22** | **58.04** | — | — |
| | | MTFA | $24.32 \pm 0.27$ | $39.64 \pm 0.22$ | $31.73 \pm 0.38$ | $51.49 \pm 0.31$ | $2.10 \pm 0.24$ | $4.07 \pm 0.45$ |
| | ✓ | ONCE | 13.6 | N/A | 17.9 | N/A | 0.7 | N/A |
| | | iMTFA | $21.67 \pm 0.27$ | $31.55 \pm 0.41$ | $27.81 \pm 0.33$ | $40.11 \pm 0.50$ | $\mathbf{3.23 \pm 0.37}$ | $\mathbf{5.89 \pm 0.61}$ |
| 5 | | Base-Only | **28.67** | **43.53** | **38.22** | **58.04** | — | — |
| | | MTFA | $26.39 \pm 0.23$ | $41.52 \pm 0.30$ | $33.11 \pm 0.22$ | $51.49 \pm 0.25$ | $\mathbf{6.22 \pm 0.59}$ | $\mathbf{11.63 \pm 1.15}$ |
| | ✓ | ONCE | 13.7 | N/A | 17.9 | N/A | 1.0 | N/A |
| | | iMTFA | $19.62 \pm 0.43$ | $28.06 \pm 0.63$ | $24.13 \pm 0.50$ | $33.69 \pm 0.75$ | $6.07 \pm 0.51$ | $11.15 \pm 0.89$ |
| 10 | | Base-Only | **28.67** | **43.53** | **38.22** | **58.04** | — | — |
| | | MTFA | $27.44 \pm 0.21$ | $42.84 \pm 0.34$ | $33.83 \pm 0.16$ | $52.04 \pm 0.19$ | $\mathbf{8.28 \pm 0.47}$ | $\mathbf{15.25 \pm 0.92}$ |
| | ✓ | ONCE | 13.7 | N/A | 17.9 | N/A | 1.2 | N/A |
| | | iMTFA | $19.26 \pm 0.30$ | $27.49 \pm 0.47$ | $23.36 \pm 0.39$ | $32.41 \pm 0.60$ | $6.97 \pm 0.49$ | $12.72 \pm 0.79$ |

Table 1: **FSOD performance on COCO for both base and novel classes.** Results include 95% confidence intervals. Inc. stands for incremental.

| Shots | Inc. | Method | Segmentation | | | | | |
|---|---|---|---|---|---|---|---|---|
| | | | Overall | | Base | | Novel | |
| | | | **AP** | **AP50** | **AP** | **AP50** | **AP** | **AP50** |
| 1 | | Base-Only | **26.34** | **41.55** | **35.12** | **55.40** | — | — |
| | | MTFA | $22.98 \pm 0.24$ | $37.48 \pm 0.35$ | $29.85 \pm 0.35$ | $48.64 \pm 0.46$ | $2.34 \pm 0.31$ | $3.99 \pm 0.51$ |
| | ✓ | iMTFA | $20.13 \pm 0.28$ | $30.64 \pm 0.41$ | $25.90 \pm 0.32$ | $39.28 \pm 0.47$ | $\mathbf{2.81 \pm 0.37}$ | $\mathbf{4.72 \pm 0.57}$ |
| 5 | | Base-Only | **26.34** | **41.55** | **35.12** | **55.40** | — | — |
| | | MTFA | $25.07 \pm 0.17$ | $39.95 \pm 0.30$ | $31.29 \pm 0.15$ | $49.55 \pm 0.20$ | $\mathbf{6.38 \pm 0.63}$ | $\mathbf{11.14 \pm 1.05}$ |
| | ✓ | iMTFA | $18.22 \pm 0.41$ | $27.10 \pm 0.61$ | $22.56 \pm 0.47$ | $33.25 \pm 0.72$ | $5.19 \pm 0.44$ | $8.65 \pm 0.68$ |
| 10 | | Base-Only | **26.34** | **41.55** | **35.12** | **55.40** | — | — |
| | | MTFA | $25.97 \pm 0.16$ | $41.28 \pm 0.25$ | $31.84 \pm 0.25$ | $50.17 \pm 0.16$ | $\mathbf{8.36 \pm 0.49}$ | $\mathbf{14.58 \pm 0.83}$ |
| | ✓ | iMTFA | $17.87 \pm 0.28$ | $26.46 \pm 0.46$ | $21.87 \pm 0.34$ | $32.01 \pm 0.57$ | $5.88 \pm 0.45$ | $9.81 \pm 0.69$ |

Table 2: **FSIS performance on COCO for both base and novel classes.** Results include 95% confidence intervals.

The worst performing super-categories are `person` and `furniture`. Aside from the large number of false negatives and background confusions, the `furniture` super-category seems to have a high number of confusions within the same super-category as well, indicated by the 'Sim' curve. This suggests iMTFA is not able to easily distinguish between classes such as `chair`, `couch` and `dining-table` given so few examples. We observe a similar trend in confusing related classes for `vehicle`, `animal` and `kitchen`.

Although the `electronic` super-category achieves the highest precision, it is only represented by the `TV` class, which was shown to be an outlier in terms of performance.

## 4. Example shots and inference results

In Figure 3, we show the $K = 5$ shots and typical inference results for iMTFA on COCO-Novel. We report on three classes: `TV`, `bird` and `person`. These classes were chosen because of their high, average and low segmentation AP, see Table 6. All examples use the same representative seed as the generated PR curves.

The `TV` class is often confused with kitchen appliances with prominent rectangular borders. This feature is uniformly seen in the $K$ available shots for this class.

The examples for the `bird` class show more variation. In this case, many of the errors are false negatives. Birds that have been correctly detected are often segmented well, as shown in our inference results. Although one of the $K$ shots is a $7 \times 7$ pixel image patch, this did not appear to reduce the robustness of our method.

Finally, the `people` class has the most varied examples, both in terms of setting and the subject's body pose. The high pose variability causes multiple detections for each person. The diverse settings in which the humans appear are likely to produce false positives similar to the bathtub classified as a human visible in the inference results.

## References


[1] Derek Hoiem, Yodsawalai Chodpathumwan, and Qieyun Dai. Diagnosing error in object detectors. In *Proceedings of the European Conference on Computer Vision (ECCV)*, pages 340–353, 2012. 1

| # | Inc. | Method | Detection | | | Segmentation | | |
|---|---|---|---|---|---|---|---|---|
| | | | **AP** | **AP50** | **AP75** | **AP** | **AP50** | **AP75** |
| 1 | | MTFA | $2.47 \pm 0.28$ | $4.85 \pm 0.52$ | $2.26 \pm 0.29$ | $2.66 \pm 0.33$ | $4.56 \pm 0.51$ | $2.77 \pm 0.38$ |
| | ✓ | iMTFA | **3.28 ± 0.35** | **6.01 ± 0.63** | **3.15 ± 0.35** | **2.83 ± 0.36** | **4.75 ± 0.58** | **2.90 ± 0.40** |
| 5 | | MRCN+FT-full | 1.3 | 3.0 | 1.1 | 1.3 | 2.7 | 1.1 |
| | | Meta R-CNN | 3.5 | 9.9 | 1.2 | 2.8 | 6.9 | 1.7 |
| | | MTFA | **6.61 ± 0.53** | **12.32 ± 1.05** | **6.39 ± 0.54** | **6.62 ± 0.54** | **11.58 ± 0.90** | **6.67 ± 0.55** |
| | ✓ | iMTFA | $6.22 \pm 0.51$ | $11.28 \pm 0.86$ | $6.01 \pm 0.52$ | $5.24 \pm 0.44$ | $8.73 \pm 0.70$ | $5.39 \pm 0.46$ |
| 10 | | MRCN+FT-full | 2.5 | 5.7 | 1.9 | 1.9 | 4.7 | 1.3 |
| | | Meta R-CNN | 5.6 | 14.2 | 3.0 | 4.4 | 10.6 | 3.3 |
| | | MTFA | **8.52 ± 0.49** | **15.53 ± 0.93** | **8.44 ± 0.51** | **8.39 ± 0.50** | **14.64 ± 0.85** | **8.46 ± 0.47** |
| | ✓ | iMTFA | $7.14 \pm 0.45$ | $12.91 \pm 0.73$ | $6.93 \pm 0.49$ | $5.94 \pm 0.43$ | $9.96 \pm 0.64$ | $6.09 \pm 0.45$ |

Table 3: **FSOD and FSIS performance on the COCO novel classes.** Results include 95% confidence intervals. Inc. stands for incremental.

| # | Inc. | Method | Detection | | | Segmentation | | |
|---|---|---|---|---|---|---|---|---|
| | | | **AP** | **AP50** | **AP75** | **AP** | **AP50** | **AP75** |
| 1 | | Siamese Mask R-CNN | 8.6 | $15.3 \pm 0.2$ | 8.8 | 6.7 | $13.5 \pm 0.2$ | 6.0 |
| | | MTFA | $8.26 \pm 0.39$ | $15.24 \pm 0.75$ | $8.11 \pm 0.34$ | $8.25 \pm 0.53$ | $14.31 \pm 0.81$ | $8.35 \pm 0.61$ |
| | ✓ | iMTFA | **10.06 ± 0.57** | **17.85 ± 0.84** | **10.05 ± 0.68** | **8.67 ± 0.59** | **15.47 ± 0.84** | **8.50 ± 0.70** |
| 5 | | Siamese Mask R-CNN | 9.4 | $16.8 \pm 0.1$ | 9.7 | 7.4 | $14.8 \pm 0.1$ | 6.7 |
| | | MTFA | **15.80 ± 0.36** | **28.12 ± 0.62** | **16.27 ± 0.56** | **15.14 ± 0.41** | **25.83 ± 0.62** | **15.90 ± 0.50** |
| | ✓ | iMTFA | $14.55 \pm 0.48$ | $25.73 \pm 0.70$ | $14.63 \pm 0.59$ | $12.33 \pm 0.41$ | $21.95 \pm 0.58$ | $12.14 \pm 0.51$ |

Table 4: **FSOD and FSIS performance on COCO-Split-2.** Results include 95% confidence intervals. The authors of Siamese Mask R-CNN only report confidence intervals for AP50.

| # | Inc. | Method | Detection | | | Segmentation | | |
|---|---|---|---|---|---|---|---|---|
| | | | **AP** | **AP50** | **AP75** | **AP** | **AP50** | **AP75** |
| 1 | | FGN | N/A | **30.8** | N/A | N/A | 16.2 | N/A |
| | | MTFA | $9.99 \pm 0.58$ | $21.68 \pm 1.21$ | $7.92 \pm 0.77$ | **9.51 ± 0.46** | **19.28 ± 1.04** | **8.69 ± 0.55** |
| | ✓ | iMTFA | **11.47 ± 0.53** | $22.41 \pm 1.03$ | **10.47 ± 0.65** | $8.57 \pm 0.56$ | $16.32 \pm 1.02$ | $8.26 \pm 0.68$ |

Table 5: **FSOD and FSIS performance on COCO2VOC.** Results include 95% confidence intervals. The authors of FGN only report confidence intervals for AP50.

| | Detection | | Segmentation | |
|---|---|---|---|---|
| | **AP** | **AP50** | **AP** | **AP50** |
| **tv** | $26.08 \pm 5.17$ | $39.16 \pm 7.66$ | $28.31 \pm 5.62$ | $39.52 \pm 7.74$ |
| **bus** | $22.35 \pm 7.18$ | $30.56 \pm 9.33$ | $23.32 \pm 7.36$ | $30.10 \pm 9.26$ |
| **car** | $11.55 \pm 4.38$ | $21.88 \pm 7.20$ | $10.85 \pm 4.07$ | $20.39 \pm 6.75$ |
| **train** | $8.74 \pm 1.90$ | $17.48 \pm 3.46$ | $10.30 \pm 2.19$ | $18.26 \pm 3.54$ |
| **airplane** | $12.34 \pm 1.90$ | $21.43 \pm 3.22$ | $8.80 \pm 1.13$ | $17.87 \pm 1.96$ |
| **sheep** | $6.73 \pm 1.92$ | $11.09 \pm 3.22$ | $5.38 \pm 1.48$ | $10.05 \pm 2.77$ |
| **couch** | $6.24 \pm 1.77$ | $11.51 \pm 3.27$ | $4.13 \pm 1.26$ | $8.47 \pm 2.33$ |
| **bottle** | $3.86 \pm 1.14$ | $8.46 \pm 2.40$ | $3.57 \pm 1.02$ | $7.70 \pm 2.09$ |
| **cow** | $4.74 \pm 1.32$ | $7.87 \pm 2.11$ | $3.48 \pm 1.04$ | $6.35 \pm 1.86$ |
| **bird** | $1.88 \pm 1.27$ | $3.46 \pm 2.32$ | $1.79 \pm 1.25$ | $3.43 \pm 2.36$ |
| **horse** | $5.12 \pm 1.47$ | $11.87 \pm 3.78$ | $1.56 \pm 0.38$ | $3.95 \pm 0.94$ |
| **chair** | $1.39 \pm 0.74$ | $3.10 \pm 1.49$ | $0.91 \pm 0.50$ | $2.26 \pm 1.14$ |
| **motorcycle** | $3.70 \pm 0.94$ | $10.70 \pm 2.41$ | $0.73 \pm 0.28$ | $2.42 \pm 0.61$ |
| **dog** | $1.61 \pm 0.81$ | $3.68 \pm 1.49$ | $0.71 \pm 0.57$ | $1.48 \pm 1.02$ |
| **boat** | $0.60 \pm 0.26$ | $1.28 \pm 0.53$ | $0.55 \pm 0.24$ | $1.28 \pm 0.56$ |
| **cat** | $5.57 \pm 1.45$ | $15.05 \pm 3.41$ | $0.17 \pm 0.11$ | $0.46 \pm 0.28$ |
| **bicycle** | $0.38 \pm 0.14$ | $1.45 \pm 0.51$ | $0.07 \pm 0.04$ | $0.40 \pm 0.22$ |
| **potted_plant** | $0.24 \pm 0.15$ | $0.82 \pm 0.46$ | $0.06 \pm 0.08$ | $0.16 \pm 0.20$ |
| **dining_table** | $0.75 \pm 0.31$ | $2.93 \pm 1.10$ | $0.02 \pm 0.01$ | $0.09 \pm 0.04$ |
| **person** | $0.47 \pm 0.14$ | $1.91 \pm 0.55$ | $0.01 \pm 0.01$ | $0.02 \pm 0.02$ |

Table 6: **FSOD and FSIS performance on the COCO novel classes, reported for every class.** Results are sorted in decreasing order of segmentation AP and include 95% confidence intervals.

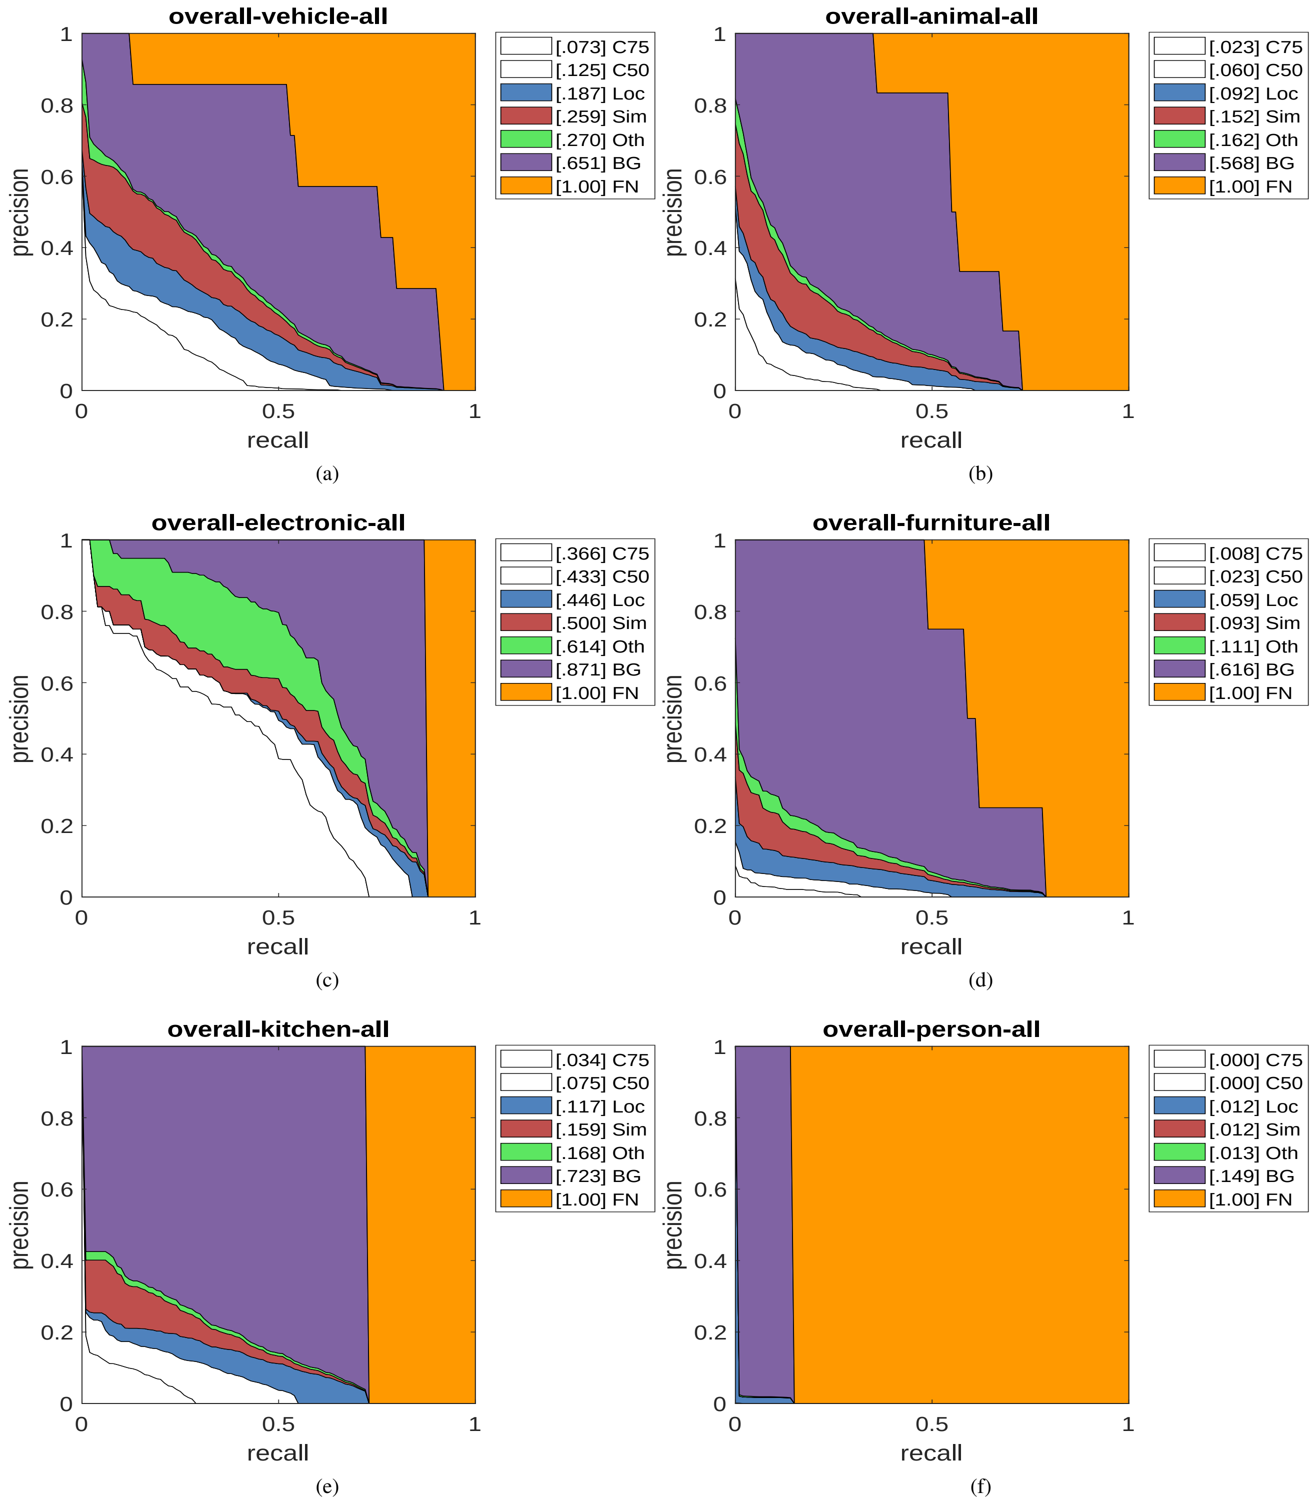


Figure 2. **Precision-Recall (PR) curves for instance segmentation on the super-categories of the COCO novel classes.** See Section 3 for an explanation of the labels.

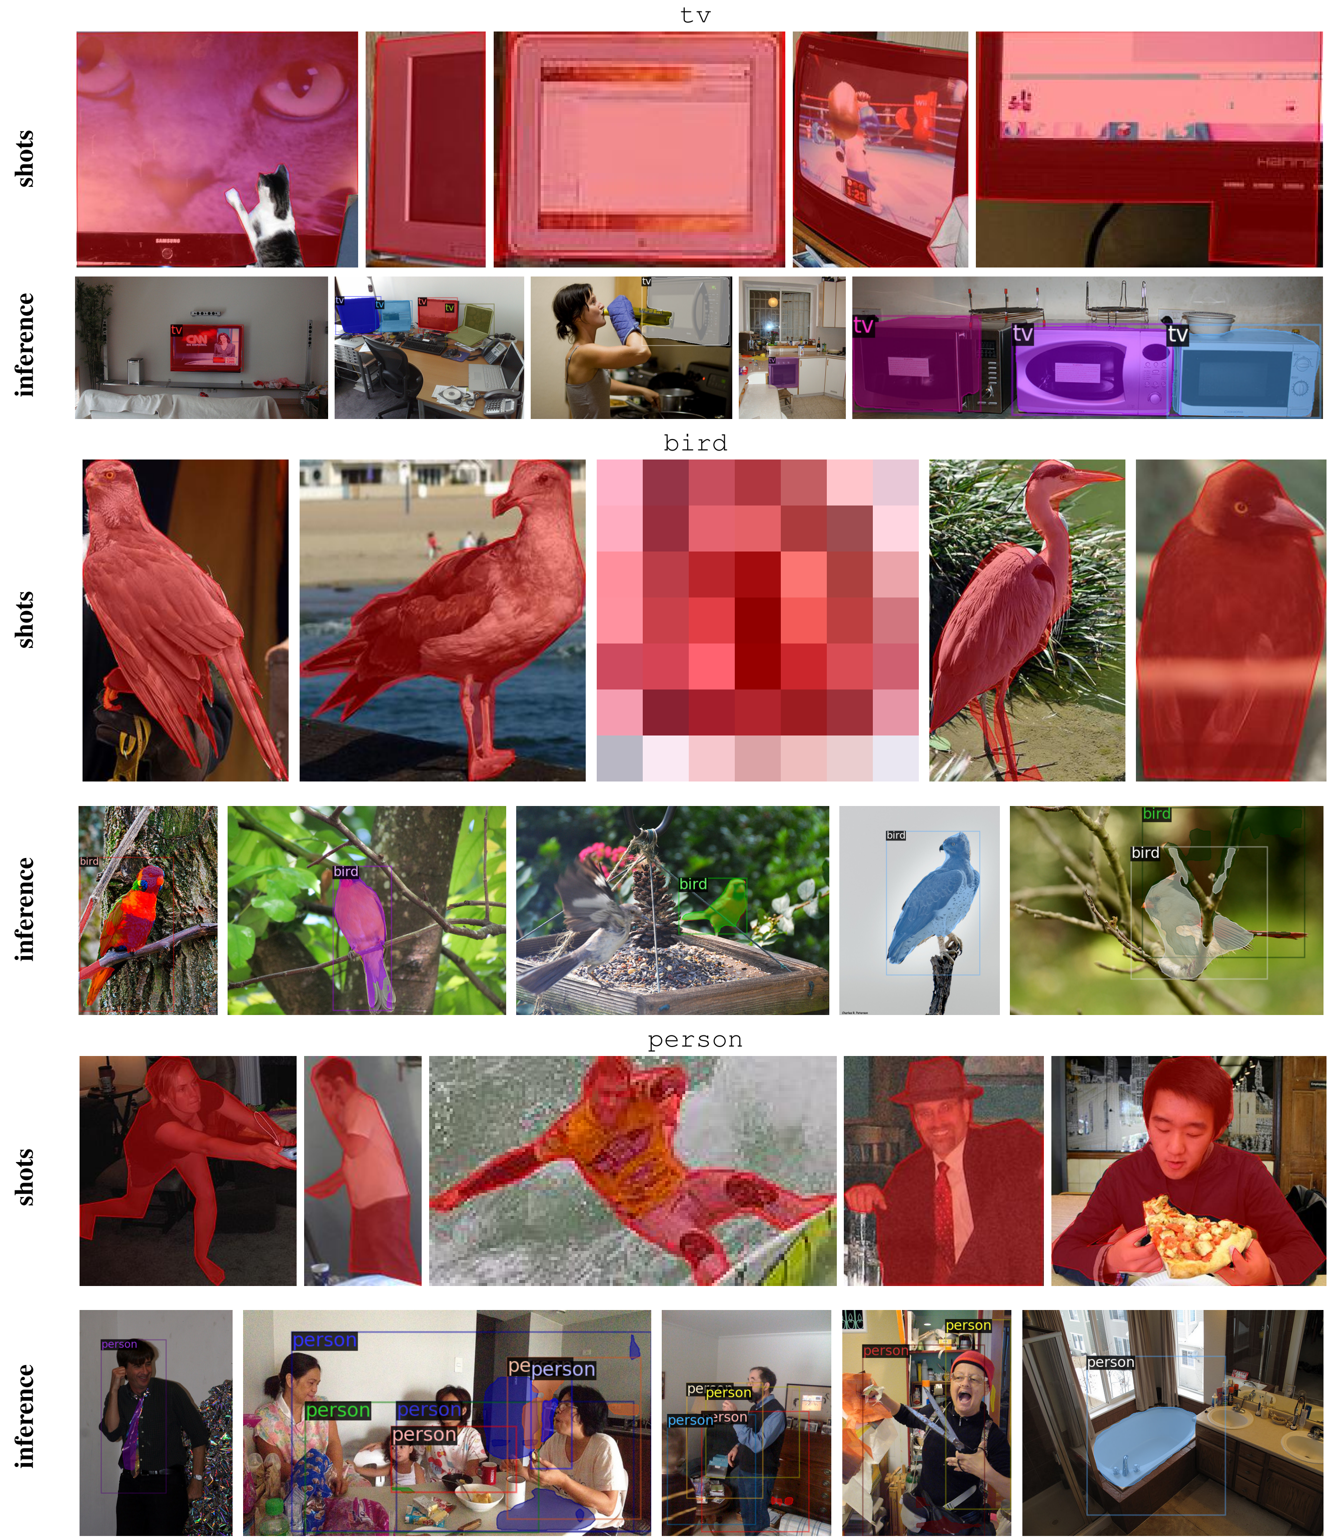


Figure 3. **Example shots and inference results.** We selected three classes with a high (`tv`), average (`bird`) and low (`person`) instance segmentation AP on COCO-Novel to demonstrate typical inference results. The objects in the $K = 5$ training shots are shown cropped. The third bird shot is a $7 \times 7$ pixel image patch.
